# Supplementary material for: Group mixing drives inequality in face-to-face gatherings
Source: arXiv:2106.11688 ancillary file (2022-03-16)
Supplement: Supplementary file 1 [file Supplementary_Material.pdf]

# Mixing dynamics and group imbalance lead to degree inequality in face-to-face interaction

## *Supplementary Material*

M. Oliveira,<sup>1\*</sup> F. Karimi,<sup>1,2</sup> M. Zens,<sup>1</sup> J. Schaible,<sup>1</sup> M. Génois,<sup>3</sup> M. Strohmaier<sup>1,4</sup>

**1** Computational Social Science, GESIS–Leibniz Institute for the Social Sciences, Germany

**2** Complexity Science Hub Vienna, Josefstädterstraße 39, 1080 Vienna, Austria

**3** Centre de Physique Théorique, Aix-Marseille University, Marseille, France

**4** Computational Social Sciences and Humanities, RWTH Aachen University, Aachen, Germany

## Contents

|          |                                                                                  |          |
|----------|----------------------------------------------------------------------------------|----------|
| <b>1</b> | <b>Data</b>                                                                      | <b>1</b> |
| 1.1      | Empirical distributions . . . . .                                                | 2        |
| 1.2      | Measuring the significant level of intra- and inter-group interactions . . . . . | 2        |
| <b>2</b> | <b>The intrinsic-attractiveness model</b>                                        | <b>3</b> |
| <b>3</b> | <b>The attractiveness–mixing model</b>                                           | <b>4</b> |
| 3.1      | Analytical derivation . . . . .                                                  | 6        |
| 3.1.1    | Comparison to simulation . . . . .                                               | 8        |
| 3.2      | Results . . . . .                                                                | 9        |
| 3.2.1    | Group differences . . . . .                                                      | 9        |
| 3.2.2    | Face-to-face characteristics . . . . .                                           | 9        |
| 3.2.3    | Asymmetric mixing . . . . .                                                      | 9        |
| 3.2.4    | Calculating $f_0^*$ . . . . .                                                    | 10       |
| 3.2.5    | Approximation of $f_0^*$ . . . . .                                               | 12       |
| 3.2.6    | Ranking inequality . . . . .                                                     | 12       |

## 1 Data

We examine six different data sets of face-to-face interaction in schools [1, 2, 3] and academic conferences [4]. Each data set contains the interactions between individuals during different social gatherings. The scheme of these data sets is as the following:

- `time stamp` – when the interaction happened,
- `pair of individuals` – the unique identification of the two individuals  $(i, j)$  involved in the interaction.

All data sets are from the SocioPatterns collaboration [5]. Table 1 provides the source of each data set. The data is generated via wearable active radio-frequency identification (RFID) proximity sensors, which captures interaction between two individuals who are facing each other within 1–1.5 meters. In each deployment of these sensors, the participants sign a term allowing the use of the data for research purposes. The participants also fill in a survey where they inform about some socio-demographic attributes. In this paper, we focus on the `gender` attribute; we denote 0 for female, 1 to male. We remove the individuals who did not fill in the survey.  $f_0$  denotes the proportional size of the minority group (i.e., female individuals) with respect to  $N$ . For each data set, we construct a network in which:

- a **node** represents an individual,
- and an **edge** indicates whether two individuals have been in face-to-face physical proximity at least once.

**Table 1:** The social networks from six different studies. The number of nodes  $N$ , the minority fraction  $f_0$ , the average degree of the minority  $\langle k_0 \rangle$ , majority  $\langle k_1 \rangle$ , overall  $\langle k \rangle$ , and the data sources.

| Data set          | $N$ | $f_0$ | $E$   | $\langle k_0 \rangle$ | $\langle k_1 \rangle$ | $\langle k \rangle$ | Ref. | URL                                                |
|-------------------|-----|-------|-------|-----------------------|-----------------------|---------------------|------|----------------------------------------------------|
| School 1 (S1)     | 242 | 0.46  | 8317  | 64.85                 | 72.08                 | 68.74               | [1]  | <a href="http://bit.ly/2ucvAUv">bit.ly/2ucvAUv</a> |
| School 2 (S2)     | 126 | 0.33  | 1710  | 24.71                 | 28.32                 | 27.14               | [2]  | <a href="http://bit.ly/37E8YtH">bit.ly/37E8YtH</a> |
| School 3 (S3)     | 180 | 0.27  | 2220  | 23.46                 | 25.11                 | 24.67               | [2]  | <a href="http://bit.ly/37E8YtH">bit.ly/37E8YtH</a> |
| School 4 (S4)     | 327 | 0.44  | 5818  | 36.48                 | 34.87                 | 35.58               | [3]  | <a href="http://bit.ly/2V2r1XF">bit.ly/2V2r1XF</a> |
| Conference 1 (C1) | 115 | 0.43  | 5508  | 95.35                 | 96.12                 | 95.79               | [4]  | <a href="http://bit.ly/2V2q7dJ">bit.ly/2V2q7dJ</a> |
| Conference 2 (C2) | 202 | 0.30  | 11412 | 118.61                | 110.56                | 112.99              | [4]  | <a href="http://bit.ly/2V2q7dJ">bit.ly/2V2q7dJ</a> |

## 1.1 Empirical distributions

In most of the networks, the degree distribution exhibits a central tendency (see Fig. 1). We replicate here also the distributions that characterize face-to-face dynamics, as previously shown in [6]. Fig. 2 depicts the distribution of interaction duration  $\Delta t$ , inter-event time  $\tau$ , and weight  $w$ . The inter-event time  $\tau$  corresponds to the amount of time that an individual  $A$  takes to interact with individual  $C$ , after having interacted with individual  $B$  immediately before. The weight  $w$  is the number of time two individuals interacted with each other.

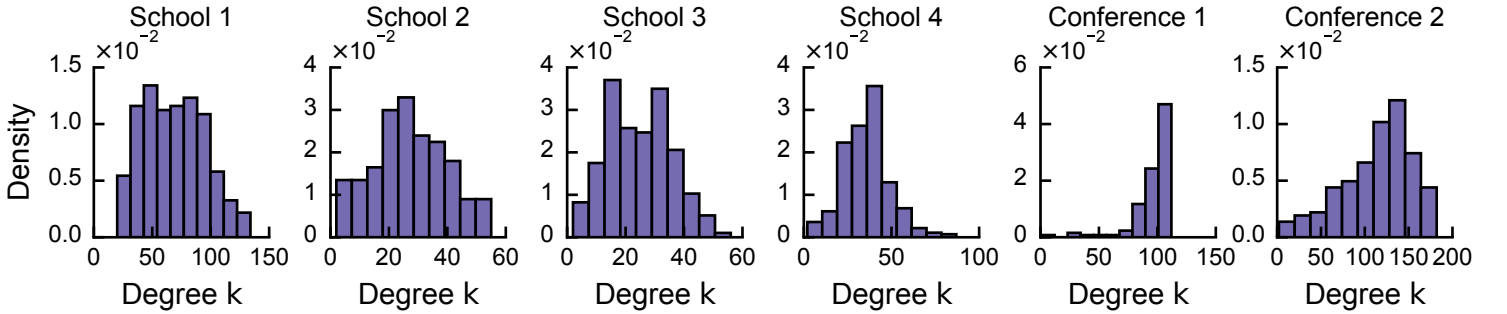

**Fig. 1:** In most of the face-to-face interaction networks, the degree distribution exhibits a central tendency.

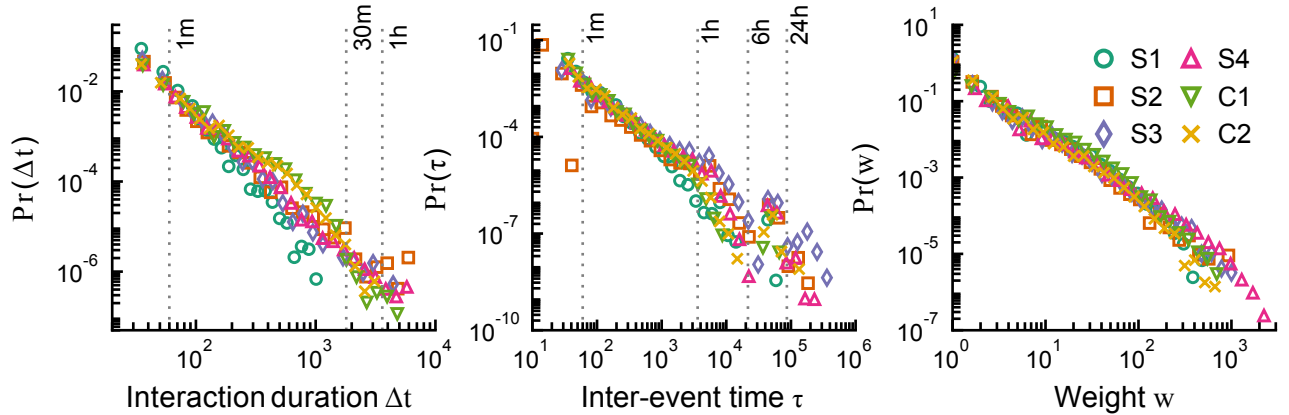

**Fig. 2:** The statistical characteristics of face-to-face interaction. The way people interact in face-to-face situations is characterized by the distributions of interaction duration, amount of time between consecutive contacts, and number of contacts between individuals.

## 1.2 Measuring the significant level of intra- and inter-group interactions

We analyze the inter- and intra-group ties in the networks by comparing them with the configuration model. We generate random networks that preserve the degree of each node in a given network and reshuffle the links, which we use to compare against the actual data [7]. Specifically, we use the implementation of the configuration model in the `networkx` library, following three steps. First, for each network, we generate  $S = 500$  random instances of the network, then we remove

the self-edges and parallel loop of the generated networks, and finally we count the number of edges  $E'_{sr}$  between groups  $r$  and  $s$  in each instance; we denote  $\overline{E'_{sr}}$  as the sample average of  $E'_{sr}$  over the  $S$  instances, and  $s(E'_{sr})$  is its standard deviation. Second, we count the number of edges between groups in the data, denoted as  $E_{sr}$ . Third, we calculate the z-score of  $E_{sr}$  with respect to  $E'_{sr}$  for each data set, defined as:

$$\text{z-score}_{sr} = \frac{E_{sr} - \overline{E'_{sr}}}{s(E'_{sr})}. \quad (1)$$

In Fig. 3, we show the z-scored distribution of  $E'_{00}$ ,  $E'_{01}$ ,  $E'_{10}$ , and  $E'_{11}$  for each data set; the vertical lines are the z-score of the respective  $E_{sr}$ .

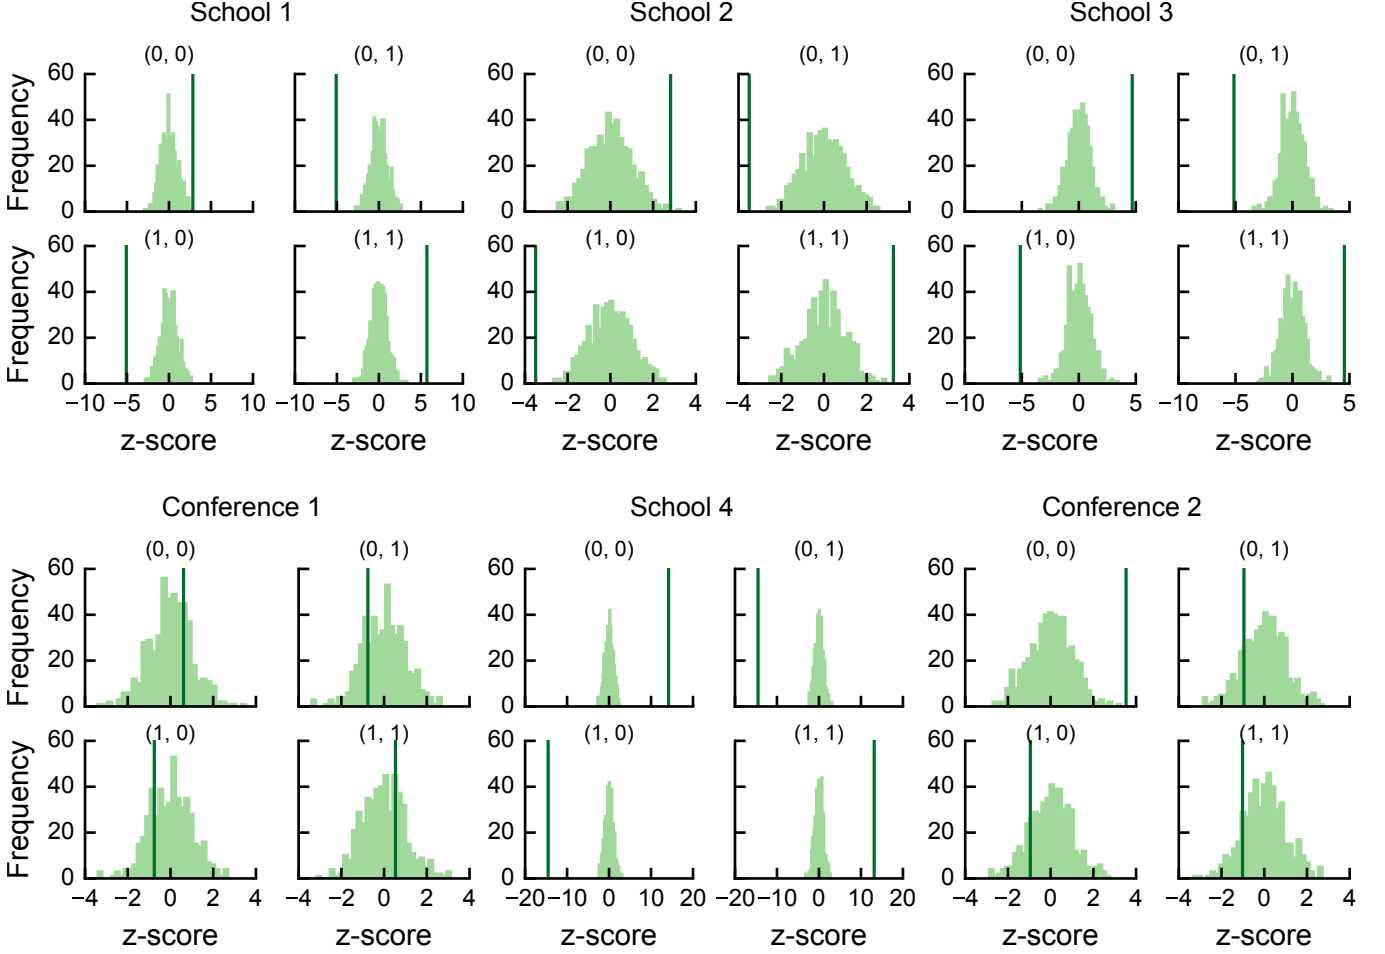

**Fig. 3:** The z-score distribution of  $E'_{rs}$  from the networks generated using the configuration model. The vertical lines are the values found in data. In most of the data sets,  $E_{rr}$  is higher than the random case, indicating that individuals tend to interact with individuals from their same group more often than random.

## 2 The intrinsic-attractiveness model

The intrinsic-attractiveness model lacks relational attributes [8], preventing it to exhibit mixing dynamics similar to data. From the data sets, we know that social groups have different average degree centrality (see Fig. 1 in the main text). Though the intrinsic-attractiveness model neglects the existence of social groups, a way that a group  $A$  would have a higher average degree than a group  $B$  is that individuals of  $A$  are more intrinsically attractive than the members of  $B$ . To analyze the mixing patterns in this situation, we simulate the intrinsic-attractiveness model in a such way that the minority has attractiveness in  $[0, 0.2]$ , whereas the majority is in  $[0.2, 1.0]$ . We run the model with different minority fraction  $f_0$ , and then we compare the network from the simulation against the configuration model (the same method of the previous section). Fig. 4 shows the mixing patterns of this experiment. If the minority group is less intrinsically attractive than

the majority, all individuals will tend to interact with the majority. That is, it is less likely for minorities to connect to minorities (i.e., the minority group does not exhibit a homophily behavior).

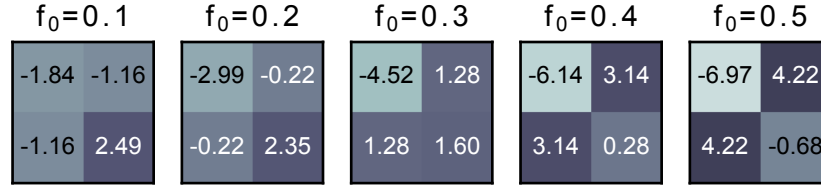

**Fig. 4:** If the minority group was intrinsically less attractive than the majority group, the minority members would tend to connect to the majority and avoid interacting with the minority.

### 3 The attractiveness–mixing model

In the attractiveness–mixing model, each individual has three attributes:

- a label  $b_i \in [0, B - 1]$ , where  $B$  is the number of groups;
- an intrinsic attractiveness  $\eta_i \in [0, 1]$ ;
- and an activation probability  $r_i \in [0, 1]$ .

In the model,  $N$  individuals perform random walks in a two-dimensional  $L \times L$  periodic space and move based on the composition of their vicinity (see Pseudocode 1). The neighborhood of an individual consists of the set of individuals

---

**Pseudocode 1:** The iteration function of the attractiveness–mixing model.

---

```

input      : list of agents individuals; mixing matrix H; neighborhood radius distance  $d$ ; move step length  $v$ 
1 Function Iteration(individuals, H,  $d$ ,  $v$ ):
2   UpdateNeighborhoods(individuals,  $d$ )
3   foreach  $i$  in individuals do
4     if IsActive( $i$ ) then
5        $k \leftarrow$  FindMostAttractiveNeighbor( $i$ ,  $d$ )
6        $\alpha_i \leftarrow 1 - \eta_k$ 
7       if  $\alpha_i > \text{Random}()$  then
8         | MoveIndividual( $i$ ,  $v$ )
9       else
10         $k \leftarrow$  FindHighestMixingNeighbor( $i$ ,  $d$ , H)
11         $\beta_i \leftarrow h_{b_i b_k}$ 
12        if  $\beta_i > \text{Random}()$  then
13          | InteractWithHighestMixingNeighbors( $i$ ,  $d$ , H)
14        end
15      end
16      if Isolated( $i$ ) then
17        if  $r_i > \text{Random}()$  then
18          | Deactivate( $i$ )
19        end
20      end
21    else
22      if  $1 - r_i > \text{Random}()$  then
23        | Activate( $i$ )
24      end
25    end
26  end

```

---

who are within radius  $d$  of that individual at time  $t$ , denoted as  $N_i(t)$ . At each time step  $t$ , each individual  $i$  moves with probability  $\alpha_i(t)$ , which embeds the intrinsic attractiveness their neighbors, and interacts with other individuals with probability  $\beta_i(t)$ , which embeds the group mixing likelihood. Precisely, an individual  $i$  moves with probability

$$\alpha_i(t) = 1 - \max_{j \in N_i(t)} \{\eta_j\} \quad (2)$$

whereas with the complementary probability the individual does not move and has the possibility to interact with individuals in  $N_i(t)$ . If an individual  $i$  does not move, this individual interacts with their neighbors of highest mixing likelihood with probability

$$\beta_i(t) = \max_{j \in N_i(t)} \{h_{b_i b_j}\}, \quad (3)$$

where  $h_{b_i b_j}$  is an element of  $\mathbf{H}$  and denotes the mixing probability between  $b_i$  and  $b_j$ . Each individual moves with a step of length  $v$  along a random direction of angle  $\xi \in [0, 2\pi)$ . Moreover, at each time step, individuals can be active or inactive, and they only move and interact with others if they are active. An inactive individual  $i$  becomes active with probability  $r_i$ , whereas an active but *isolated* individual  $i$  becomes inactive with probability  $1 - r_i$ .

In our simulations, we initialize the individuals in random positions within  $L \times L$ , and their activation probability  $r_i$  and intrinsic attractiveness  $\eta_i$  are set by drawing from a continuous uniform distribution in  $[0, 1]$ . In the initialization, the individuals are activated with probability 0.5. Pseudocode 1 describes an iteration in the model.

The functions in the code are defined as the following:

- `Isolated( $i, d$ )`: returns `False` if there are individuals within radius  $d$  from individual  $i$ , otherwise returns `True`.
- `IsActive( $i$ )`: returns `True` if individual  $i$  is active, otherwise returns `False`.
- `Activate( $i$ )`: activates individual  $i$ .
- `Deactivate( $i$ )`: deactivates individual  $i$ .
- `MoveIndividual( $i, v$ )`: moves individual  $i$  with a step  $v$  towards a random angle  $\xi \in [0, 2\pi)$ .
- `FindMostAttractiveNeighbor( $i, d$ )`: returns the identifier of the most attractive neighbor of individual  $i$  within radius  $d$ .
- `FindHighestMixingNeighbor( $i, d, \mathbf{H}$ )`: returns the identifier of the neighbor of individual  $i$  within radius  $d$  with the highest mixing probability, given a mixing matrix  $\mathbf{H}$ .
- `InteractWithHighestMixingNeighbors( $i, d, \mathbf{H}$ )`: individual  $i$  interacts with their neighbors (within radius  $d$ ) of highest mixing probability, given mixing matrix  $\mathbf{H}$ .
- `Random()`: returns a random number from a uniform distribution in  $[0, 1]$ .

Finally, Table 2 summarizes the main entities in the model and paper.

**Table 2:** Variables, constants, and notations of the model.

| Entity       | Description                                    |
|--------------|------------------------------------------------|
| $E$          | Number of edges in a network (or system)       |
| $N$          | Number of nodes in a network (or system)       |
| $B$          | Number of node groups in a network (or system) |
| $n_r$        | Number of nodes in group $r$                   |
| $f_r$        | Group fraction, defined as $n_r/N$             |
| $E_{rs}$     | Number of edges between group $r$ and $s$      |
| $e_{rs}$     | Normalized edge count, defined as $E_{rs}/E$   |
| $\mathbf{H}$ | The mixing matrix                              |
| $b_i$        | The group label of the individual $i$          |
| $r_i$        | Individual $i$ 's activation probability       |
| $\eta_i$     | Individual $i$ 's attractiveness               |
| $v$          | Step length                                    |
| $L$          | Space size                                     |

### 3.1 Analytical derivation

Here we derive the normalized group edge matrix and the mixing matrix for the attractiveness–mixing model. Let us assume that we have two groups of nodes labeled as group 0 and group 1. The normalized elements of the mixing matrix tell us the probability of finding inter- or intra-group edges in the network. Here we are interested in calculating the probability of intragroup links for group 0, denoted by  $e_{00}$ , but the analytic derivations for group 1 follows a similar logic. The definition of  $e_{00}$  is as the following:

$$e_{00} = \frac{E_{00}}{E_{00} + E_{01} + E_{10} + E_{11}}, \quad (4)$$

where  $E_{rs}$  denotes total number of edges between group  $r$  and  $s$ . We assume that individuals' attractiveness, denoted by  $\eta$ , is drawn from a uniform distribution. We denote the group mixing in the model by  $h$ . Note that group mixing can be asymmetrical in its nature (e.g., the tendency of nodes of group 0 to attach to nodes of group 1 could be larger than the tendency of nodes of group 1 to interact to group 0). To keep the derivations general, we denote group mixing between nodes of group 0 by  $h_{00}$  and group mixing between nodes of group 1 is  $h_{11}$ . If group mixing is symmetric, we have  $h_{00} = h_{11} = h$ .

In the model, the probability of two individuals of the same type to interact in a cell space depends on the group size, group mixing, and individuals' attractiveness. Specifically, the probability of an individual  $i$  from group 0 to interact with an individual  $j$  from group 0 is:

$$p_{ij} = f_0^2 h_{00} \eta_j, \quad (5)$$

where  $f_0$  denotes fraction of nodes of group 0 and  $\eta_j$  is the attractiveness of node  $j$ . Note that the two dimensional area in which nodes are interacting  $L \times L$  and the diameter range in which each individual decides to stay or move,  $d$ , only determine the density of the network and do not affect the interaction probabilities. To simplify the derivation, we assume a situation of low spatial density of agents, so that almost all situations of potential interaction involve only two agents, and that non-pairwise interactions are negligible (i.e., the dilute system hypothesis).

Let  $N$  be the total number of agents. Due to the activation process, at one time  $t$  the number of active nodes is on average:

$$N_a = \langle r_i \rangle N$$

as in the dilution hypothesis there should not be any correlation between  $r_i$  and the fact that the agent is isolated.

The agents are gathered in two groups labeled 0 and 1, with proportions  $f_0$  and  $f_1$  such as  $f_0 \leq f_1$ . The number of active nodes in each group are thus:

$$N_0 = f_0 N_a \quad \text{and} \quad N_1 = f_1 N_a.$$

The model generates a *temporal network*, in which nodes are the agents and interactions between them are edges, which are created and destroyed as time passes. Let  $E_t$  be the number of edges created in the whole network during a time step  $\Delta t$ . As the connecting behavior is independent from time, the total number of edges in the network after a time  $T$  is simply:

$$E_T = E_t \times \frac{T}{\Delta t}.$$

Let us express the number of new edges created at time  $t$  in each component. We focus first on edges between two agents from group 0. Consider an agent  $i$  from group 0:

- In the dilution hypothesis, the probability  $p_0$  to find an agent  $j$  from group 0 in the vicinity of agent  $i$  is simply related to the surface of the vicinity and the density  $\rho_0$  of agents from group 0 on the field:

$$p_0 = \rho_0 S = \frac{N_0}{L} \pi d^2 = \frac{f_0 N_a}{L} \pi d^2 = f_0 \rho_a \pi d^2$$

with  $\rho_a$  the density of active agents.

- To have an interaction, *both* agents needs to be available and not move away. As we consider only pairwise interactions, the probability for one agent to be available is simply the attractiveness of the other agent. The probability to have an interaction is thus the product of both attractivenesses:  $\gamma = \eta_i \eta_j$ .

- If interacting, the probability for agent  $i$  to interact with agent  $j$  is then simply  $h_{00}$  as both are from group 0 and there are no other agents in the vicinity.

The process of edge creation is agent-centered. Therefore, 3 situations lead to the creation of an edge between an agent  $i$  and an agent  $j$ :

1. agent  $i$  only initiates the creation;
2. agent  $j$  only initiates the creation;
3. both agents initiates the creation.

All three cases lead to the same result: an single edge created between agents  $i$  and  $j$ . The probability for the edge to appear is thus:  $p_{ij} = p_{i \rightarrow j} + p_{j \rightarrow i} + p_{i \leftrightarrow j}$ . In the case of two agents of group 0, this probability is on average:

$$\begin{aligned} p_{ij,00} &= f_0 \rho_a \pi d^2 \times \gamma \times (h_{00}(1 - h_{00}) + (1 - h_{00})h_{00} + h_{00}^2) \\ &= f_0 \rho_a \pi d^2 \gamma (2h_{00} - h_{00}^2) \\ &= f_0 \rho_a \pi d^2 \gamma (1 - h_{01}^2) \end{aligned}$$

by replacing  $h_{00}$  with  $1 - h_{01}$ . Indeed, the probability to have an edge between two nodes of group 0 is the probability to not have both nodes choosing to not connect. Finally, the number of edges within group 0 created during one time step is then:

$$\begin{aligned} E_{00} &= \frac{N_0}{2} p_{ij,00} \\ &= \frac{f_0 N_a}{2} f_0 \rho_a \pi d^2 \gamma (1 - h_{01}^2) \\ &= \frac{N_a^2 \pi d^2}{2L} \gamma f_0^2 (1 - h_{01}^2) \end{aligned}$$

with the  $1/2$  factor taking into account double counting. Similarly, we get for the other components:

$$\begin{aligned} E_{11} &= \frac{N_a^2 \pi d^2}{2L} \gamma f_1^2 (1 - h_{10}^2) \\ E_{10} &= \frac{N_a^2 \pi d^2}{L} \gamma f_1 f_0 (1 - h_{00} h_{11}) \\ E_{01} &= \frac{N_a^2 \pi d^2}{L} \gamma f_0 f_1 (1 - h_{00} h_{11}) \end{aligned}$$

The  $1/2$  factor is absent form the  $E_{01}$  and  $E_{10}$  components as there is no double counting in these cases. However, these two components count the same population of edges, so we need only to consider one of them. The total number of edges created is then:

$$E = \frac{N_a^2 \pi d^2}{2L} \gamma \left( f_0^2 (1 - h_{01}^2) + f_1^2 (1 - h_{10}^2) + 2f_0 f_1 (1 - h_{00} h_{11}) \right),$$

Note that since attractiveness values are drawn from the same distribution for all the nodes, the product of the values,  $\gamma$ , remains intact. Finally, the shares of edges for each component are:

$$\begin{aligned} e_{00} &= \frac{f_0^2 (1 - h_{01}^2)}{f_0^2 (1 - h_{01}^2) + f_1^2 (1 - h_{10}^2) + 2f_0 f_1 (1 - h_{00} h_{11})} \\ e_{11} &= \frac{f_1^2 (1 - h_{10}^2)}{f_0^2 (1 - h_{01}^2) + f_1^2 (1 - h_{10}^2) + 2f_0 f_1 (1 - h_{00} h_{11})} \\ e_{10} = e_{01} &= \frac{f_0 f_1 (1 - h_{00} h_{11})}{f_0^2 (1 - h_{01}^2) + f_1^2 (1 - h_{10}^2) + 2f_0 f_1 (1 - h_{00} h_{11})} \end{aligned}$$

Since the process of edge creation is on average constant in time, these shares are also constant on average.

### 3.1.1 Comparison to simulation

Our analytical expressions describe well the model. To show that, we simulate the model using different parameters values ( $h_{rr}$  and  $f_0$ ) and compared against the analytical prediction. Fig. 5 and Fig. 6 depict this comparison, showing that our analytical expressions predicts the normalized number of edges in the simulation and the mixing matrix.

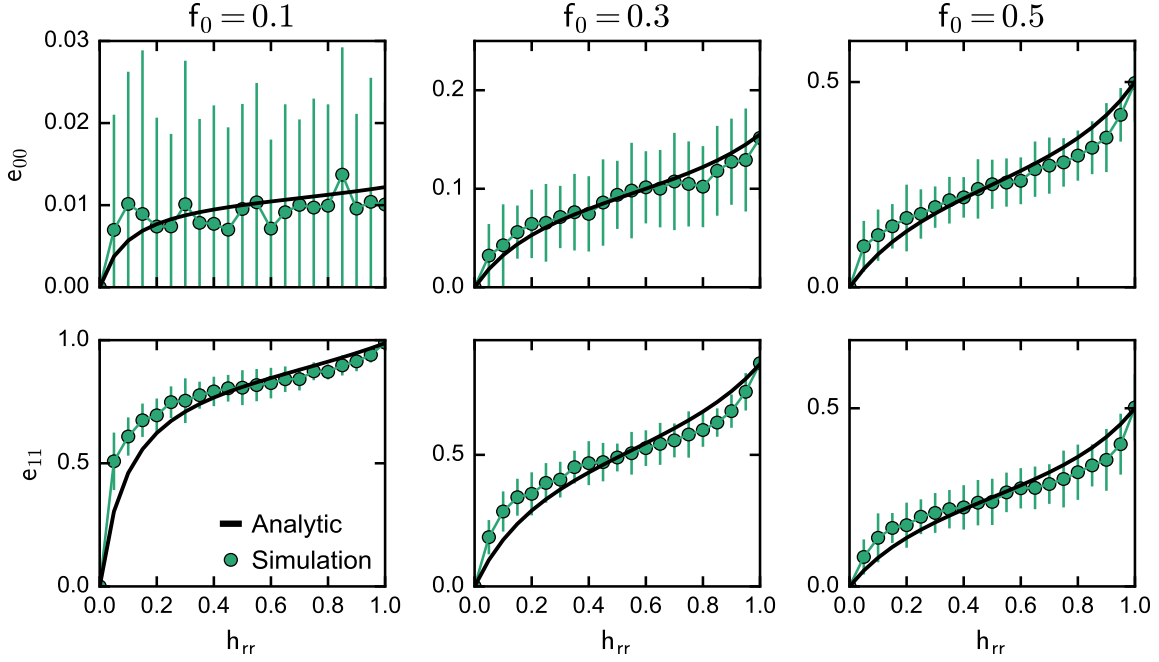

**Fig. 5:** Our analytical expressions predict well the number of edges inter- and intra-group.

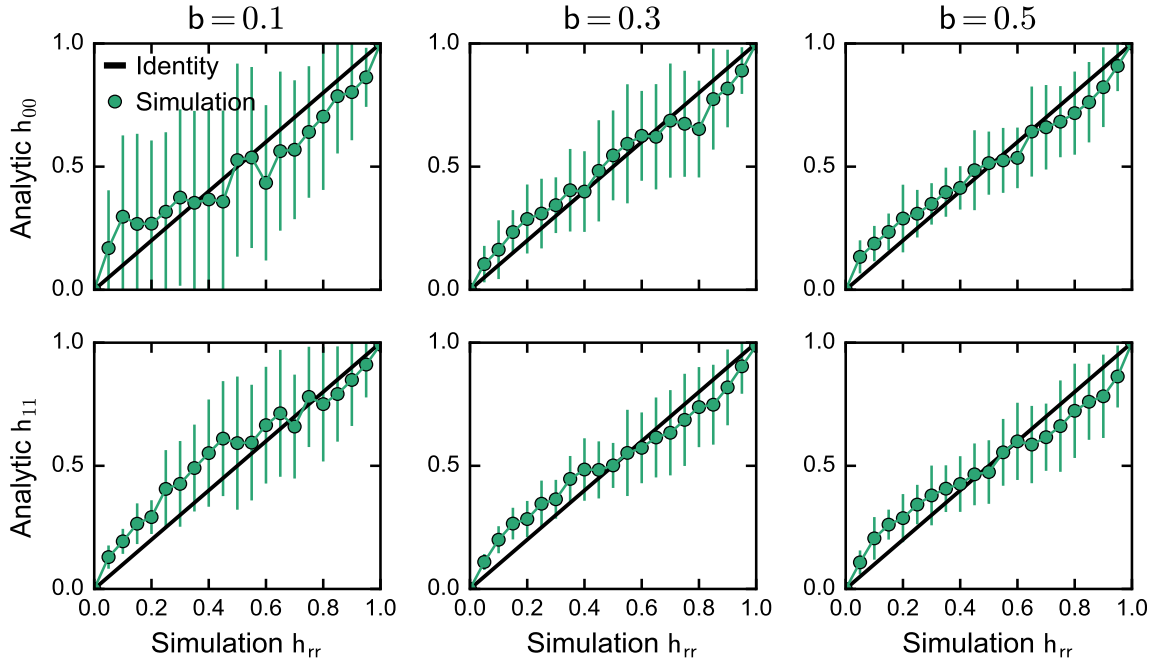

**Fig. 6:** Our analytical expressions enable us to extract the mixing matrix  $\mathbf{H}$  from data. First, we simulate the model with a range values of  $h_{rr}$ , then we estimate  $h_{rr}$  from the final simulation.

## 3.2 Results

### 3.2.1 Group differences

Our model reproduces the group differences found in data. We simulate the model with the parameters as estimated from the data (see Fig. 1 in the main text). For each data set, we simulate our model 50 times using the following parameters:  $L = 100$ ,  $d = 1$ ,  $v = 1$ , and  $N$  same as the data set. To show that our model reproduce degree differences, for each simulation, we measure the average degree of the whole network  $\langle k \rangle$  and the average group degree of the minority, denoted as  $\langle k_0 \rangle$ , and majority,  $\langle k_1 \rangle$ . We compare each group  $r$  with the whole network using  $z$  scores, defined as  $(\langle k_r \rangle - \langle k \rangle) / s[k]$ , where  $s[k]$  is the standard deviation of  $k$ . We compare these differences with the data sets (Fig. 7) using Kolmogorov–Smirnov test for each simulation separately. Table 3 shows how many times  $p > .05$  in the 50 simulations for each data set and each group.

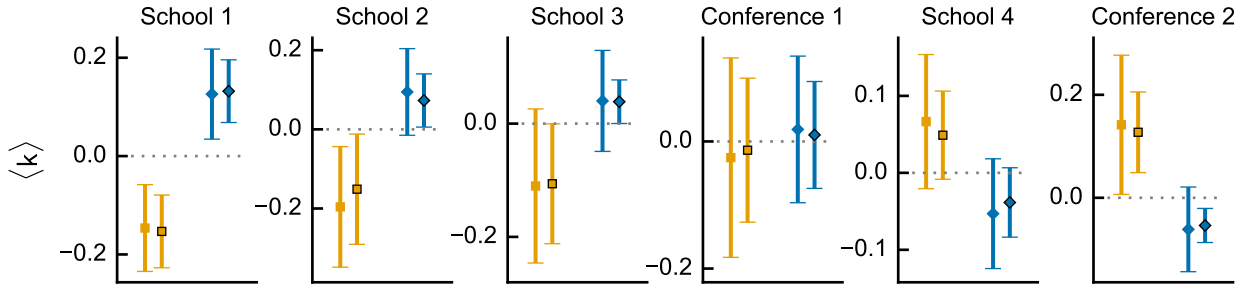

**Fig. 7:** The  $z$  scores of group degrees in simulations and data sets.

**Table 3:** Kolmogorov–Smirnov test between data and each of the 50 simulation runs.

| Data set     | Minority | Majority |
|--------------|----------|----------|
| School 1     | 50/50    | 50/50    |
| School 2     | 46/50    | 50/50    |
| School 3     | 50/50    | 49/50    |
| Conference 1 | 41/50    | 42/50    |
| School 4     | 48/50    | 50/50    |
| Conference 2 | 50/50    | 50/50    |

### 3.2.2 Face-to-face characteristics

Our model emulates the statistical characteristics of face-to-face interaction. First, we simulate our model, then we measure the interaction duration, the inter-event time, and the weight of the interactions in our model simulations. As shown in Fig. 8, the model has a behavior similar to what it is found in data. Note that the intrinsic-attractiveness model also emulates these statistics, as shown in [8].

### 3.2.3 Asymmetric mixing

We investigate the regimes in the model with asymmetric mixing by analyzing the whole parameter space of the model. This analysis is performed following two steps. First, we estimate the average minority degree for different values of  $h_{00}$  and  $h_{11}$ , given specific minority fraction values  $f_0 \in \{0.1, 0.2, 0.3, 0.4, 0.5\}$ . Second, we measure the distance of the minority group degree to the average degree, denoted as  $k_0 - \langle k \rangle$ , using  $z$ -scores, depicted in Fig. 9. Note that, when  $f_0 < 0.5$ , the majority mixing  $h_{11}$  explains most of the variance of  $k_0 - \langle k \rangle$ . To verify this, we measure the standard deviation of  $k_0 - \langle k \rangle$  given a fixed  $h_{00}$  over different values of  $h_{11}$ , and vice-versa. Fig. 10 depicts this standard deviation over different values of  $f_0$ , showing that  $h_{11}$  dominates the changes in  $k_0 - \langle k \rangle$ .

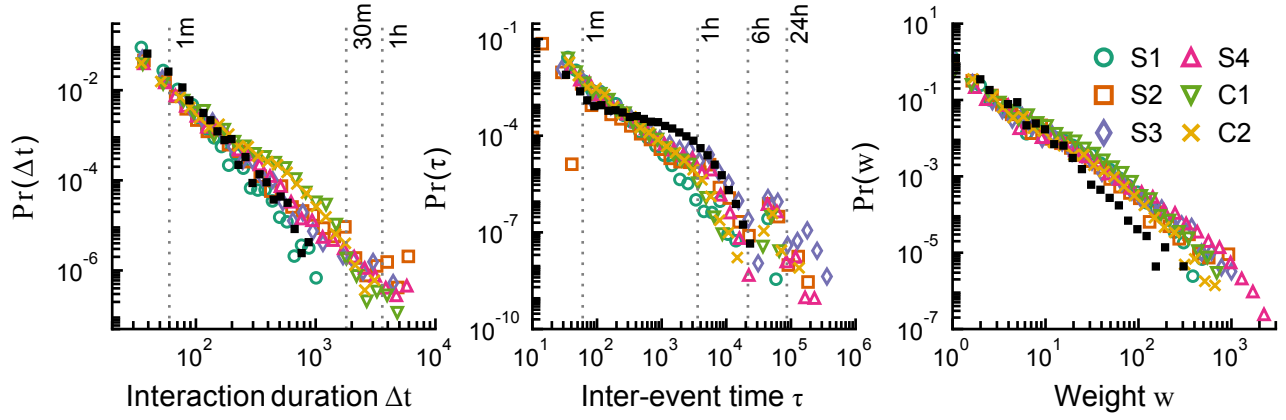

**Fig. 8:** The attractiveness–mixing model (solid black rectangles) shows similar characteristics found in face-to-face situations.

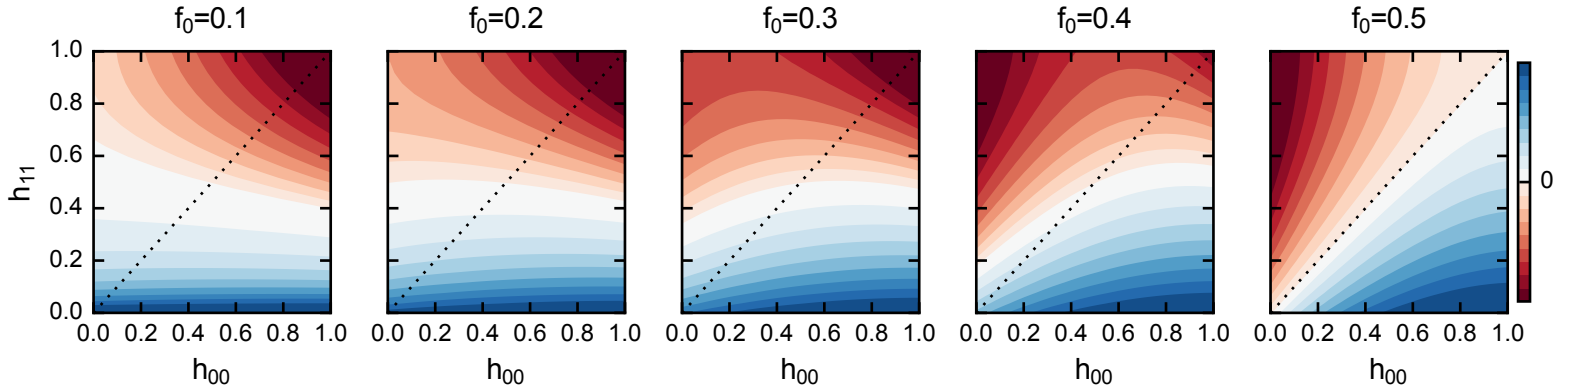

**Fig. 9:** The z-score distance of the minority group degree to the average degree ( $k_0 - \langle k \rangle$ ) over the whole parameter space ( $h_{00}, h_{11}$ ), given different minority sizes.

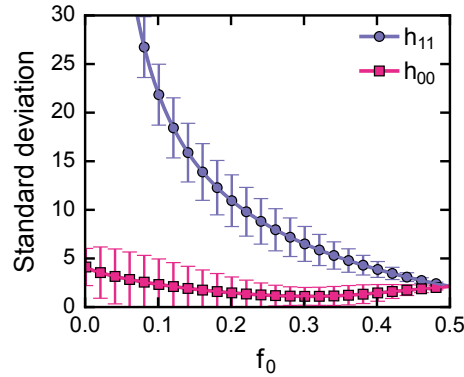

**Fig. 10:** Most of the changes in  $k_0 - \langle k \rangle$  is given by  $h_{11}$ . In the plot, the standard deviation of  $k_0 - \langle k \rangle$  given a fixed  $h_{00}$  value over different values of  $h_{11}$  (circles) and the standard deviation of  $k_0 - \langle k \rangle$  given a fixed  $h_{11}$  value over different values of  $h_{00}$  (squares).

### 3.2.4 Calculating $f_0^*$

As shown in the main text, an increase of the minority mixing  $h_{00}$  can have an opposite impact on degree inequality, depending on the minority fraction; Fig. 11A shows different cases of that. To understand these contrasting impacts, we examine the derivative of  $k_0 - \langle k \rangle$  with respect to  $h_{00}$  as a function of  $f_0$ . Precisely, we are interested in derivative of the

following relationship:

$$\begin{aligned} \langle k_0 \rangle \frac{N_0}{E} &= 2e_{00} + e_{01} + e_{10} \\ &= \frac{2f_0^2(1 - (1 - h_{00})^2) + 2(1 - f_0)f_0(1 - h_{11}h_{00})}{2f_0(1 - f_0)(1 - h_{11}h_{00}) + f_0^2(1 - (1 - h_{00})^2) + (1 - (1 - h_{11})^2)(1 - f_0)^2}, \end{aligned} \quad (6)$$

with respect to  $h_{00}$ , which is given by:

$$\begin{aligned} \frac{d}{dh_{00}} \left[ \langle k_0 \rangle \frac{N_0}{E} \right] &= \frac{4f_0^2(1 - h_{00}) - 2h_{11}(1 - f_0)f_0}{2f_0(1 - f_0)(1 - h_{11}h_{00}) + f_0^2(1 - (1 - h_{00})^2) + (1 - (1 - h_{11})^2)(1 - f_0)^2} \\ &\quad - \frac{(2f_0^2(1 - h_{00}) - 2h_{11}(1 - f_0)f_0)(2f_0^2(1 - (1 - h_{00})^2) + 2(1 - f_0)f_0(1 - h_{11}h_{00}))}{(2f_0(1 - f_0)(1 - h_{11}h_{00}) + f_0^2(1 - (1 - h_{00})^2) + (1 - (1 - h_{11})^2)(1 - f_0)^2)^2}. \end{aligned} \quad (7)$$

We highlight that this function depends on  $h_{00}$  and  $h_{11}$  because both remain in the derivative, as shown in Fig. 11B for different values of  $h_{00}$  and  $h_{11}$ . We find the zero of this function, denoted  $f_0^*$ , which tells us the critical minority size at which the transition seen in Fig. 11A takes place. We find that this fraction is given by:

$$f_0^* = \frac{\sqrt{-(h_{11} - 2)h_{11}^2(2h_{11}h_{00} - h_{11} + 2h_{00}^2 - 6h_{00} + 4) - h_{11}^2(h_{00} + 1) + h_{11}^3 + 2h_{11}(h_{00} - 1)}}{-2h_{11}^2h_{00} + h_{11}^3 + h_{11}(h_{00}^2 + 4h_{00} - 4) - 2h_{00} + 2}. \quad (8)$$

We use Eq. (8) to find when increasing minority homophily is always beneficial to the minority group regardless of  $h_{11}$ . Specifically, we characterize the upper limit of  $f_0^*$ , denoted as  $\bar{f}_0^*$ , which represents the smallest minority size in which

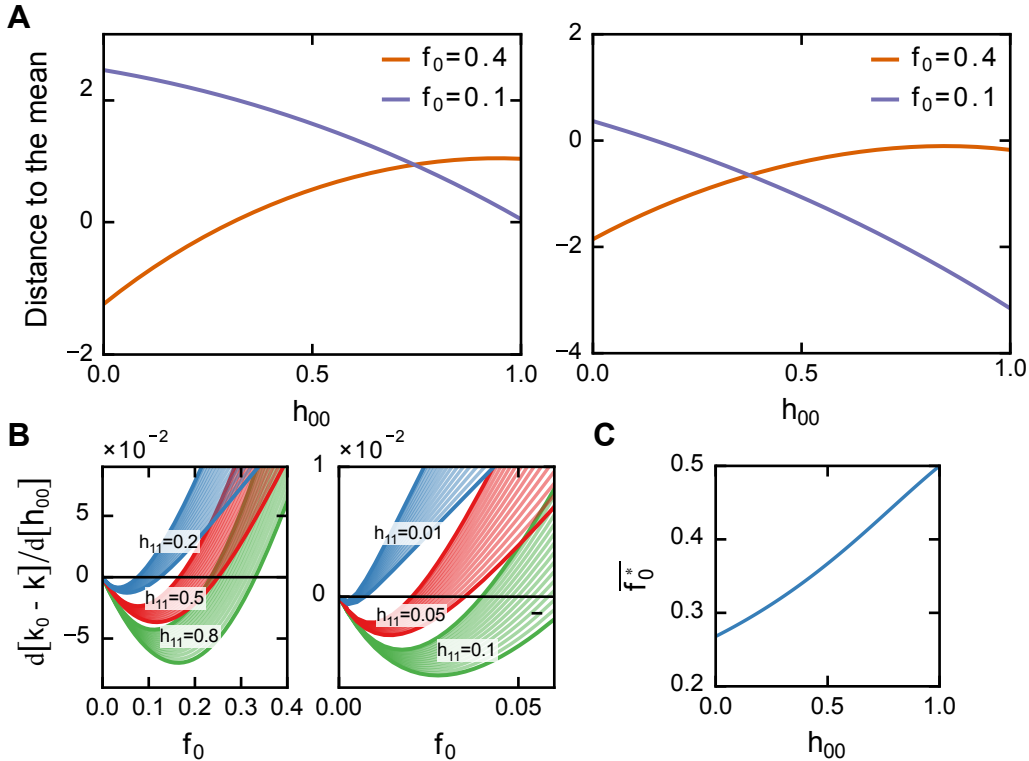

**Fig. 11:** (A) Increasing the minority mixing  $h_{00}$  can lead to opposite impacts on degree inequality. (B) The derivative of  $k_0 - \langle k \rangle$  with respect to  $h_{00}$  as a function of  $f_0$ . Note that the derivative also depends on  $h_{00}$  and  $h_{11}$ . In each plot, different colors represent different values of  $h_{11}$ . Curves with the same color are different values of  $h_{00}$ . The dashed lines are guides for the zero of each curve. (C) The upper limit of the critical minority size, denoted as  $\bar{f}_0^*$ , represents the smallest minority size in which the minority group can increase its homophily without detriment to its average degree, given  $h_{00}$  and regardless of the majority mixing  $h_{11}$ .

the minority group can increase its homophily without detriment to its average degree, regardless of the majority mixing. This upper limit is equivalent to the critical size  $f_0^*$  when  $h_{11} = 1$ , thus we simplify Eq. (8), finding:

$$\overline{f_0^*} = \frac{1}{2 - h_{00} + \sqrt{3 + 2(h_{00} - 2)h_{00}}}, \quad (9)$$

as shown in Fig. 11C. We note that in all the derivations above, we investigate  $f_0^*$  as a function of group mixing  $e$ .

### 3.2.5 Approximation of $f_0^*$

We find an approximation of Eq. (8) by ignoring the denominator of Eq. (6).

$$\begin{aligned} \frac{d}{dh_{00}} [\langle k_0 \rangle - \langle k \rangle] &= \frac{d}{dh_{00}} \left[ \frac{(2E_{00} + E_{01})}{f_0 N} - \frac{2E_{00} + 2E_{01} + 2E_{11}}{N} \right] = 0 \\ &\Rightarrow 2E'_{00}(1 - f_0) + E'_{01}(1 - 2f_0) = 0 \end{aligned} \quad (10)$$

If we assume that

$$\frac{d}{dh_{00}} [(f_0^2(1 - h_{01}^2) + 2f_0f_1(1 - h_{00}h_{11}) + f_1^2(1 - h_{10}^2))] = 0,$$

we have:

$$2E'_{00}(1 - f_0) + E'_{01}(1 - 2f_0) = 2(2f_0h_{01})f_1 + -2f_0f_1h_{11}(1 - 2f_0) = 0. \quad (11)$$

Rearranging Eq. (11), we get:

$$f_0^* = \frac{h_{11}}{2(h_{01} + h_{11})}. \quad (12)$$

Note that same result can be achieved by ignoring higher order terms of homophily ( $h \ll 1$ ) in Eq. (8). This approximation works the best when the values of  $h_{00}$  and  $h_{11}$  are not at their extremes. We measured the error of the approximation, finding that the error is below 0.01 in most of the cases (see Fig. 12). That is, the critical minority fraction can be underestimated or overestimated by less than 1% when  $h_{00}$  and  $h_{11}$  are not extreme values.

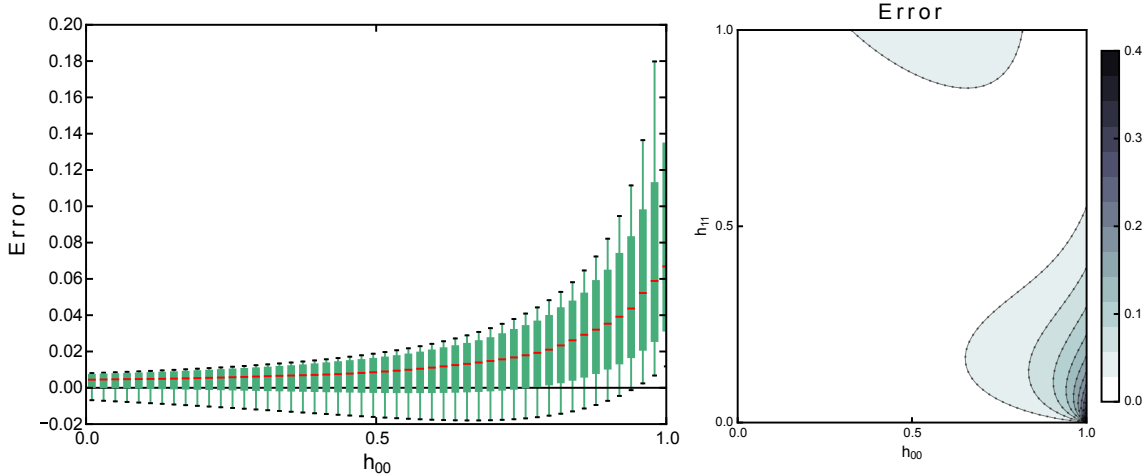

**Fig. 12:** Approximation error.

### 3.2.6 Ranking inequality

As shown in the main text, when we rank individuals by degree, we incorporate the mixing dynamics into the rank. A position in the degree rank is a result of group and individual attributes. Depending on the system regime, the rank can have over- or under-representation of minorities. To investigate minority representation, we rank individuals separately by degree and attractiveness, and then we compare the representation of minorities in each rank. We measure the minority representation (i.e., percentage) in the rank as we increased the rank length (i.e., the top-k rank). Given that the

attractiveness is uniformly distributed, we expect that the number of minority members in the top-k rank is proportional to the minority group size. We find this exact behavior when we rank individuals by attractiveness (Fig. 13). In the case of the degree rank, however, minority members are only represented correctly in the extreme case of rank-size equals to the number of individuals.

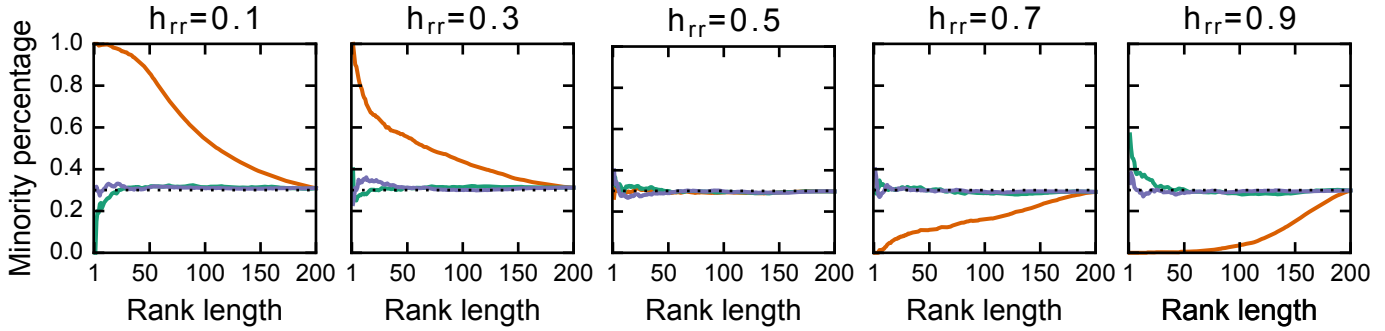

**Fig. 13:** While the minority group is over-represented in degree ranks in heterophilic regimes, it is under-represented in homophilic regimes. The adjusted rank accounts for the difference in the mixing and decreases the bias in ranks, regardless of  $h_{rr}$ .

## References

- [1] Juliette Stehlé, Nicolas Voirin, Alain Barrat, Ciro Cattuto, Lorenzo Isella, Jean-François Pinton, Marco Quaggiotto, Wouter Van den Broeck, Corinne Régis, Bruno Lina, and Philippe Vanhems. High-Resolution Measurements of Face-to-Face Contact Patterns in a Primary School. *PLoS ONE*, 6(8):e23176, aug 2011.
- [2] Julie Fournet and Alain Barrat. Contact Patterns among High School Students. *PLoS ONE*, 9(9):e107878, sep 2014.
- [3] Rossana Mastrandrea, Julie Fournet, and Alain Barrat. Contact patterns in a high school: A comparison between data collected using wearable sensors, contact diaries and friendship surveys. *PLoS ONE*, 10(9):e0136497, 09 2015.
- [4] Mathieu Génois, Maria Zens, Clemens Lechner, Beatrice Rammstedt, and Markus Strohmaier. Building connections: How scientists meet each other during a conference. *arXiv preprint arXiv:1901.01182*, 2019.
- [5] SocioPatterns. <http://www.sociopatterns.org/>. Accessed: 2020-02-25.
- [6] Ciro Cattuto, Wouter van den Broeck, Alain Barrat, Vittoria Colizza, Jean François Pinton, and Alessandro Vespignani. Dynamics of person-to-person interactions from distributed RFID sensor networks. *PLoS ONE*, 5(7):1–9, 2010.
- [7] Sergei Maslov and Kim Sneppen. Specificity and stability in topology of protein networks. *Science*, 296(5569):910–913, 2002.
- [8] Michele Starnini, Andrea Baronchelli, and Romualdo Pastor-Satorras. Modeling human dynamics of face-to-face interaction networks. *Physical Review Letters*, 110(16):1–5, 2013.
